# Supplementary material for: Randomized linear algebra for model reduction. Part I: Galerkin methods and error estimation
Source: arXiv:1803.02602 source file (2019-10-31)
Supplement: Supplementary file 1 [file SUPPLEMENTARY_MATERIAL.pdf]

# Supplementary material for the article "Randomized linear algebra for model reduction. Part I: Galerkin methods and error estimation", by O. Balabanov and A. Nouy, published in Advances in Computational Mathematics, 2019.

Oleg Balabanov*† and Anthony Nouy*‡

Here we provide detailed proofs of Remark 3.8 and of some statements used in the proofs of Propositions 3.7 and 3.9 in [2].

## 1 Supplementary material for the proof of [2, Proposition 3.7]

In the proof of [2, Proposition 3.7] for the complex case (i.e., $\mathbb{K} = \mathbb{C}$) we used the following result.

**Proposition 1.1.** *Let $\boldsymbol{\Theta}$ be a real random matrix. If $\boldsymbol{\Theta}$ is $(\varepsilon, \delta, 2d)$ oblivious $\ell_2 \to \ell_2$ subspace embedding for subspaces of vectors in $\mathbb{R}^n$, then it is $(\varepsilon, \delta, d)$ oblivious $\ell_2 \to \ell_2$ subspace embedding for subspaces of vectors in $\mathbb{C}^n$.*

*Proof of Proposition 1.1.* Let $V \subset \mathbb{C}^n$ be a $d$-dimensional subspace with a basis $\{\mathbf{v}_i\}_{i=1}^d$. Let us introduce a real subspace $W = \mathrm{span}(\{\mathrm{Re}(\mathbf{v}_i)\}_{i=1}^d) + \mathrm{span}(\{\mathrm{Im}(\mathbf{v}_i)\}_{i=1}^d)$. Observe that

$$\mathrm{Re}(\mathbf{v}) \text{ and } \mathrm{Im}(\mathbf{v}) \in W, \quad \forall \mathbf{v} \in V.$$

Consequently, if $\boldsymbol{\Theta}$ is an $\varepsilon$-embedding for $W$, then

$$| \|\mathrm{Re}(\mathbf{v})\|^2 - \|\boldsymbol{\Theta}\mathrm{Re}(\mathbf{v})\|^2 | \leq \varepsilon \|\mathrm{Re}(\mathbf{v})\|^2, \quad \forall \mathbf{v} \in V, \tag{1a}$$

$$| \|\mathrm{Im}(\mathbf{v})\|^2 - \|\boldsymbol{\Theta}\mathrm{Im}(\mathbf{v})\|^2 | \leq \varepsilon \|\mathrm{Im}(\mathbf{v})\|^2, \quad \forall \mathbf{v} \in V. \tag{1b}$$

Since $\boldsymbol{\Theta}$ is a real matrix, relations (1) imply

$$| \|\mathbf{v}\|^2 - \|\boldsymbol{\Theta}\mathbf{v}\|^2 | \leq \varepsilon \|\mathbf{v}\|^2, \quad \forall \mathbf{v} \in V. \tag{2}$$

By definition of $\boldsymbol{\Theta}$ and the fact that $\dim(W) \leq 2d$, it follows that $\boldsymbol{\Theta}$ is an $\varepsilon$-embedding for $W$ with probability at least $1 - \delta$. From this we deduce that (2) holds with probability at least $1 - \delta$. It remains to show that (2) implies

$$|\langle \mathbf{x}, \mathbf{y} \rangle - \langle \boldsymbol{\Theta}\mathbf{x}, \boldsymbol{\Theta}\mathbf{y} \rangle| \leq \varepsilon \|\mathbf{x}\| \|\mathbf{y}\|, \quad \forall \mathbf{x}, \mathbf{y} \in V. \tag{3}$$

Let $\mathbf{x}, \mathbf{y} \in V$ be any two vectors from $V$. Define $\mathbf{x}^* := \mathbf{x}/\|\mathbf{x}\|$, $\mathbf{y}^* := \mathbf{y}/\|\mathbf{y}\|$ and

$$\omega := \frac{\langle \mathbf{x}^*, \mathbf{y}^* \rangle - \langle \boldsymbol{\Theta}\mathbf{x}^*, \boldsymbol{\Theta}\mathbf{y}^* \rangle}{|\langle \mathbf{x}^*, \mathbf{y}^* \rangle - \langle \boldsymbol{\Theta}\mathbf{x}^*, \boldsymbol{\Theta}\mathbf{y}^* \rangle|}.$$

*Centrale Nantes, LMJL, UMR CNRS 6629, France.
†Polytechnic University of Catalonia, LaCàn, Spain.
‡Corresponding author (anthony.nouy@ec-nantes.fr).

Observe that $|\omega| = 1$ and $\langle \mathbf{x}^*, \omega \mathbf{y}^* \rangle - \langle \mathbf{\Theta x}^*, \omega \mathbf{\Theta y}^* \rangle$ is a real number. Then, (2) and the parallelogram identity yield

$$\begin{aligned}
4|\langle \mathbf{x}^*, \mathbf{y}^* \rangle - \langle \mathbf{\Theta x}^*, \mathbf{\Theta y}^* \rangle| &= |4\langle \mathbf{x}^*, \omega \mathbf{y}^* \rangle - 4\langle \mathbf{\Theta x}^*, \omega \mathbf{\Theta y}^* \rangle| \\
&= |\|\mathbf{x}^* + \omega \mathbf{y}^*\|^2 - \|\mathbf{x}^* - \omega \mathbf{y}^*\|^2 + 4\mathrm{Im}(\langle \mathbf{x}^*, \omega \mathbf{y}^* \rangle) \\
&- \big(\|\mathbf{\Theta}(\mathbf{x}^* + \omega \mathbf{y}^*)\|^2 - \|\mathbf{\Theta}(\mathbf{x}^* - \omega \mathbf{y}^*)\|^2 + 4\mathrm{Im}(\langle \mathbf{\Theta x}^*, \omega \mathbf{\Theta y}^* \rangle)\big)\,| \\
&= |\|\mathbf{x}^* + \omega \mathbf{y}^*\|^2 - \|\mathbf{\Theta}(\mathbf{x}^* + \omega \mathbf{y}^*)\|^2 - \big(\|\mathbf{x}^* - \omega \mathbf{y}^*\|^2 - (\|\mathbf{\Theta}(\mathbf{x}^* - \omega \mathbf{y}^*)\|^2\big) \\
&+ 4\mathrm{Im}(\langle \mathbf{x}^*, \omega \mathbf{y}^* \rangle - \langle \mathbf{\Theta x}^*, \omega \mathbf{\Theta y}^* \rangle)| \\
&\le \varepsilon \|\mathbf{x}^* + \omega \mathbf{y}^*\|^2 + \varepsilon \|\mathbf{x}^* - \omega \mathbf{y}^*\|^2 = 4\varepsilon.
\end{aligned}$$

The relation (3) follows immediately. □

## 2 Supplementary material for [2, Remark 3.8]

Recall that $\mathbf{\Theta} \in \mathbb{C}^{k \times n}$ is called a rescaled complex Gaussian matrix if

$$\mathbf{\Theta} := \frac{1}{\sqrt{2}}(\mathbf{\Theta}_{\mathrm{Re}} + j\mathbf{\Theta}_{\mathrm{Im}}), \tag{4}$$

where $\mathbf{\Theta}_{\mathrm{Re}}$, $\mathbf{\Theta}_{\mathrm{Im}}$ are two independent rescaled real Gaussian matrices (that have i.i.d. entries with mean 0 and variance $k^{-1}$). Let us now give a proof of the statement in [2, Remark 3.8] (see proposition below).

**Proposition 2.1.** *A distribution of rescaled complex Gaussian matrices (defined by (4)) with $k \ge 3.94\varepsilon^{-2}(13.8d + \log(1/\delta))$ rows satisfies $(\varepsilon, \delta, d)$ oblivious $\ell_2 \to \ell_2$ subspace embedding property.*

The proof of this statement shall be obtained by following the proof of [2, Proposition 3.7] updating the constants in some places. First, let us establish the following result.

**Lemma 2.2.** *A rescaled complex Gaussian matrix $\mathbf{\Theta}$ (defined by (4)) with $k \ge (\varepsilon^2/2 - \varepsilon^3/3)^{-1}\log(2/\delta)$ is a $(\varepsilon, \delta, 1)$ oblivious $\ell_2 \to \ell_2$ subspace embedding.*

*Proof of Lemma 2.2.* Let $\mathbf{z} \in \mathbb{C}^n$ be an arbitrary unit vector. Define $\mathbf{x} := \begin{bmatrix} \mathrm{Re}(\mathbf{z}) \\ -\mathrm{Im}(\mathbf{z}) \end{bmatrix}$, $\mathbf{y} := \begin{bmatrix} \mathrm{Im}(\mathbf{z}) \\ \mathrm{Re}(\mathbf{z}) \end{bmatrix}$ and $\mathbf{\Theta}^* := [\mathbf{\Theta}_{\mathrm{Re}}, \mathbf{\Theta}_{\mathrm{Im}}]$. Observe that $\mathbf{\Theta}^*$ is a rescaled real Gaussian matrix, $\mathbf{x}$ and $\mathbf{y}$ are orthogonal unit vectors, and

$$\|\mathbf{\Theta z}\|^2 = \frac{1}{2}\|\mathbf{\Theta}^* \mathbf{x}\|^2 + \frac{1}{2}\|\mathbf{\Theta}^* \mathbf{y}\|^2.$$

Since products of a Gaussian matrix with orthogonal unit vectors are independent Gaussian vectors, consequently, $k\mathbf{\Theta}^*\mathbf{x}$ and $k\mathbf{\Theta}^*\mathbf{y}$ are independent $k$-dimensional standard Gaussian vectors. We conclude that $2k\|\mathbf{\Theta z}\|^2$ has a chi-squared distribution with $2k$ degrees of freedom. Finally, the standard tail-bounds for chi-squared distribution ensure that

$$|\|\mathbf{\Theta z}\|^2 - 1| > \varepsilon,$$

holds with probability less than $\delta = 2\exp(-k(\varepsilon^2/2 - \varepsilon^3/3))$, which completes the proof. □

*Proof of Proposition 2.1.* We can use a similar proof as the one of [2, Proposition 3.7] for the real case. Let $V \subset \mathbb{C}^n$ be a $d$-dimensional subspace and let $\mathcal{S} = \{\mathbf{x} \in W : \|\mathbf{x}\| = 1\}$ be the unit sphere of $V$. By the volume argument it follows that for any $\gamma > 0$ there exists a $\gamma$-net $\mathcal{N}$ of $\mathcal{S}$ satisfying $\#\mathcal{N} \le (1 + 2/\gamma)^{2d}$. For $\eta$ such that $0 < \eta < 1/2$, let $\mathbf{\Theta} \in \mathbb{C}^{k \times n}$ be a rescaled complex Gaussian matrix (defined by (4)) with $k \ge 3\eta^{-2}(4d\log(1 + 2/\gamma) + \log(1/\delta))$ rows. By Lemma 2.2 and a union bound argument, we have that

$$\{\ |\|\mathbf{x} + \mathbf{y}\|^2 - \|\mathbf{\Theta}(\mathbf{x} + \mathbf{y})\|^2| \le \eta\|\mathbf{x} + \mathbf{y}\|^2, \quad \forall \mathbf{x}, \mathbf{y} \in \mathcal{N}\}$$

holds with probability at least $1-\delta$. This implies that

$$\{ \ |\langle \mathbf{x}, \mathbf{y} \rangle - \langle \mathbf{\Theta x}, \mathbf{\Theta y} \rangle| \le \eta, \quad \forall \mathbf{x}, \mathbf{y} \in \mathcal{N} \} \tag{5}$$

holds with probability at least $1-\delta$.

Assume that $\gamma < 1$. It can be shown that any vector $\mathbf{n} \in \mathcal{S}$ can be expressed as $\mathbf{n} = \sum_{i \ge 0} \alpha_i \mathbf{n}_i$, where $\mathbf{n}_i \in \mathcal{N}$ and $\alpha_i$ are real coefficients such that $0 \le \alpha_i \le \gamma^i$. The proof of this fact directly follows the one for the real case in the proof of [2, Proposition 3.7]. Then (5) implies that for all $\mathbf{n} \in \mathcal{S}$,

$$\begin{aligned} \|\mathbf{\Theta n}\|^2 &= \sum_{i,j \ge 0} \langle \mathbf{\Theta n}_i, \mathbf{\Theta n}_j \rangle \alpha_i \alpha_j \\ &\le \sum_{i,j \ge 0} (\langle \mathbf{n}_i, \mathbf{n}_j \rangle \alpha_i \alpha_j + \eta \alpha_i \alpha_j) = 1 + \eta (\sum_{i \ge 0} \alpha_i)^2 \le 1 + \frac{\eta}{(1-\gamma)^2}, \end{aligned}$$

and, similarly, $\|\mathbf{\Theta n}\|^2 \ge 1 - \frac{\eta}{(1-\gamma)^2}$. Therefore, (5) implies

$$|1 - \|\mathbf{\Theta n}\|^2| \le \eta/(1-\gamma)^2, \quad \forall \mathbf{n} \in \mathcal{S}. \tag{6}$$

For any $\varepsilon \le 0.5/(1-\gamma)^2$ let us choose $\eta = (1-\gamma)^2 \varepsilon$. Now we use the argument from the proof of Proposition 1.1, which states that (2) yields (3). This result implies that, if (6) is satisfied, then $\mathbf{\Theta}$ is a $\ell_2 \to \ell_2$ $\varepsilon$-subspace embedding for $V$. We have that if $k \ge 3\varepsilon^{-2}(1-\gamma)^{-4}(4d\log(1 + 2/\gamma) + \log(1/\delta))$, then (5) (and as a consequence (6)) holds with probability at least $1-\delta$, which means that $\mathbf{\Theta}$ is $(\varepsilon, \delta, d)$ oblivious $\ell_2 \to \ell_2$ subspace embedding. As in [2, Proposition 3.7] the lower bound for $k$ is attained with $\gamma = 0.0656$.

□

# 3 Supplementary material for the proof of [2, Proposition 3.9]

Let us now present a proof of [3, Lemma 4.3] and [6, Theorem 3.1] for the complex case and with improved constants (see Proposition 3.1), which is used in the proof of [2, Proposition 3.9]. Consider a SRHT matrix $\mathbf{\Theta}$ of size $k \times n$, with $n$ being a power of 2. Recall that

$$\mathbf{\Theta} = k^{-1/2}(\mathbf{R}\mathbf{H}_n\mathbf{D}), \tag{7}$$

where $\mathbf{R}$ are the first $k$ rows of a random permutation of rows of the identity matrix, $\mathbf{H}_n$ is a Hadamard matrix, and $\mathbf{D}$ is a random diagonal matrix with i.i.d. entries with Rademacher distribution (i.e., taking values $\pm 1$ with equal probabilities). To be consistent with the notations from [6, 3] let us also define a rescaled Hadamard matrix $\mathbf{H} := \frac{1}{\sqrt{n}}\mathbf{H}_n$ with orthonormal columns.

**Proposition 3.1** (Complex version of Lemma 4.3 in [3], Theorem 3.1 in [6])**.** *Let $\mathbf{V} \in \mathbb{C}^{n \times d}$ be a matrix with orthonormal columns. Let $0 < \varepsilon < 1$ and $0 < \delta < 1$. Draw at random a matrix $\mathbf{\Theta}$ defined in (7) with*

$$k \ge 2(\varepsilon^2 - \varepsilon^3/3)^{-1}[\sqrt{d} + \sqrt{8\log(n/\delta)}]^2 \log(d/\delta).$$

*Then with probability at least $1-3\delta$, the singular values of $\mathbf{\Theta V}$ belong to the interval $[\sqrt{1-\varepsilon}, \sqrt{1+\varepsilon}]$.*

Proposition 3.1 can be derived from complex extensions of [6, Lemmas 3.3 and 3.4] presented below.

**Lemma 3.2** (Lemma 3.3 in [6])**.** *Let $\mathbf{V} \in \mathbb{C}^{n \times d}$ be a matrix with orthonormal columns. Draw at random a diagonal matrix $\mathbf{D}$ in (7). The rows $\mathbf{w}_j^{\mathrm{T}}$ of $\mathbf{HDV}$ satisfy*

$$\mathbb{P}(\max_{j=1,\dots,n} \|\mathbf{w}_j\| \le \sqrt{\frac{d}{n}} + \sqrt{\frac{8\log(n/\delta)}{n}}) \ge 1-\delta.$$

*Proof of Lemma 3.2.* This lemma can be proven with exactly the same steps as in the proof of [6, Lemma 3.3]. We have $\mathbf{w}_j = \mathbf{V}^{\mathrm{T}}\mathrm{diag}(\mathbf{i})\mathbf{H}\mathbf{e}_j$ where $\mathbf{e}_j$ is the $j$th column of the identity matrix and $\mathbf{i}$ is a Rademacher vector. Define functions $f_j(\mathbf{x}) := \|\mathbf{V}^{\mathrm{T}}\mathrm{diag}(\mathbf{x})\mathbf{H}\mathbf{e}_j\|$. Observe that $f_j(\mathbf{x}) = \|\mathbf{V}^{\mathrm{T}}\mathbf{E}_j\mathbf{x}\|$, with $\mathbf{E}_j := \mathrm{diag}(\mathbf{H}\mathbf{e}_j)$ being a matrix with 2-norm $\|\mathbf{E}_j\| = \frac{1}{\sqrt{n}}$. We have,

$$\forall \mathbf{x}, \mathbf{y},\ |f_j(\mathbf{x}) - f_j(\mathbf{y})| \le \|\mathbf{V}^{\mathrm{T}}\mathbf{E}_j(\mathbf{x}-\mathbf{y})\| \le \|\mathbf{V}\|\|\mathbf{E}_j\|\|\mathbf{x}-\mathbf{y}\| = \frac{1}{\sqrt{n}}\|\mathbf{x}-\mathbf{y}\|.$$

Moreover, the functions $f_j(\mathbf{x})$ are convex, which allows to apply the Rademacher tail bound [6, Proposition 2.1]

$$\mathbb{P}(f_j(\mathbf{i}) \ge \mathbb{E}f_j(\mathbf{i}) + \frac{1}{\sqrt{n}}t) \le \exp\left(-t^2/8\right),\ \forall t \ge 0, \tag{8}$$

with $\mathbf{i}$ being a Rademacher vector. Observe that $\mathbb{E}f_j(\mathbf{i}) \le (\mathbb{E}(f_j(\mathbf{i}))^2)^{1/2} = \|\mathbf{E}_j\mathbf{V}\|_F \le \|\mathbf{E}_j\|\|\mathbf{V}\|_F = \sqrt{\frac{d}{n}}$. The statement of the proposition follows by combining this relation with (8) with $t = \sqrt{8\log(n/\delta)}$, and by using the union bound argument. □

**Lemma 3.3** (Lemma 3.4 in [6])**.** *Let $\mathbf{W} \in \mathbb{C}^{n\times d}$ have orthonormal columns. Let $0 < \varepsilon < 1$ and $0 < \delta < 1$. Let $\mathbf{w}_j^{\mathrm{T}}$ denote the rows of $\mathbf{W}$ and let $M := n\max_{j=1,\dots,n}\|\mathbf{w}_j\|^2$. Draw at random a permutation matrix $\mathbf{R}$ in (7) with*

$$k \ge 2(\varepsilon^2 - \varepsilon^3/3)^{-1}M\log(d/\delta).$$

*Then with probability at least $1-2\delta$, all the singular values of $\sqrt{\frac{n}{k}}\mathbf{R}\mathbf{W}$ belong to the interval $[\sqrt{1-\varepsilon}, \sqrt{1+\varepsilon}]$.*

To prove Lemma 3.3 we shall use the matrix Chernoff tail bounds from [6]. For any Hermitian matrix $\mathbf{X}$, let $\lambda_{\min}(\mathbf{X})$ and $\lambda_{\max}(\mathbf{X})$ denote the minimal and the maximal eigenvalues of $\mathbf{X}$.

**Theorem 3.4** (Theorem 2.2 in [6])**.** *Consider a finite set $X \subseteq \mathbb{C}^{d\times d}$ of Hermitian positive semi-definite matrices. Define the constant $L := \max_{\mathbf{X}_j\in X}\lambda_{\max}(\mathbf{X}_j)$. Let $\{\mathbf{X}_i\}_{i=1}^k \subseteq X$ be a uniformly sampled, without replacement, random subset of $X$ and $\mathbf{X} := \sum_{i=1}^k \mathbf{X}_i$. Then*

$$\mathbb{P}(\lambda_{\min}(\mathbf{X}) \le (1-\varepsilon)\mu_{\min}) \le d\left(\frac{e^{-\varepsilon}}{(1-\varepsilon)^{1-\varepsilon}}\right)^{\mu_{\min}/L},$$

$$\mathbb{P}(\lambda_{\max}(\mathbf{X}) \ge (1+\varepsilon)\mu_{\max}) \le d\left(\frac{e^{\varepsilon}}{(1+\varepsilon)^{1+\varepsilon}}\right)^{\mu_{\max}/L},$$

*where $\mu_{\min} = k\ \lambda_{\min}(\mathbb{E}\mathbf{X}_1)$ and $\mu_{\max} = k\ \lambda_{\max}(\mathbb{E}\mathbf{X}_1)$.*

*Proof of Theorem 3.4.* The proof directly follows the one in [6], since all the ingredients used in the proof of [6, Theorem 2.2] (which are [7, Proposition 3.1, Lemma 3.4, Lemma 5.8] and the result of [4]) are formulated for (Hermitian) positive semi-definite matrices. □

*Proof of Lemma 3.3.* Define $X := \{\mathbf{w}_j\mathbf{w}_j^{\mathrm{H}}\}_{j=1}^n$. Consider the matrix

$$\mathbf{X} := (\mathbf{R}\mathbf{W})^{\mathrm{H}}\mathbf{R}\mathbf{W} = \sum_{j\in T}\mathbf{w}_j\mathbf{w}_j^{\mathrm{H}},$$

where $T$ is a set, with $\#T = k$, of elements of $\{1, 2, \dots, n\}$ drawn uniformly and without replacement. The matrix $\mathbf{X}$ can be written as

$$\mathbf{X} = \sum_{i=1}^k \mathbf{X}_i,$$

where $\{\mathbf{X}_i\}_{i=1}^k$ is a uniformly drawn, without replacement, random subset of $X$. We have $\mathbb{E}(\mathbf{X}_1) = \frac{1}{n}\mathbf{W}^{\mathrm{H}}\mathbf{W} = \frac{1}{n}\mathbf{I}$. Furthermore,

$$\lambda_{\max}(\mathbf{w}_j\mathbf{w}_j^{\mathrm{H}}) = \|\mathbf{w}_j\|^2 \leq \frac{M}{n},\ 1 \leq j \leq n.$$

By applying Theorem 3.4 and some algebraic operations, we obtain

$$\mathbb{P}(\lambda_{\min}(\mathbf{X}) \leq (1-\varepsilon)k/n) \leq d\left(\frac{e^{-\varepsilon}}{(1-\varepsilon)^{1-\varepsilon}}\right)^{k/M} \leq d\ e^{-(\varepsilon^2/2-\varepsilon^3/6)k/M} \leq \delta,$$

$$\mathbb{P}(\lambda_{\max}(\mathbf{X}) \geq (1+\varepsilon)k/n) \leq d\left(\frac{e^{\varepsilon}}{(1+\varepsilon)^{1+\varepsilon}}\right)^{k/M} \leq d\ e^{-(\varepsilon^2/2-\varepsilon^3/6)k/M} \leq \delta.$$

The statement of the lemma follows by a union bound argument. □

*Proof of Proposition 3.1.* Let $\mathbf{W} = \mathbf{HDV}$. Observe that $\mathbf{W}$ has orthonormal columns. The statement of the proposition follows from Lemma 3.2 with the tail bound from Lemma 3.3 and a union bound argument. □

# References


[1] D. Achlioptas. Database-friendly random projections: Johnson-lindenstrauss with binary coins. *Journal of computer and System Sciences*, 66(4):671–687, 2003.

[2] O. Balabanov and A. Nouy. Randomized linear algebra for model reduction. Part I: Galerkin methods and error estimation. *Advances in Computational Mathematics*, 2019.

[3] C. Boutsidis and A. Gittens. Improved matrix algorithms via the subsampled randomized hadamard transform. *SIAM Journal on Matrix Analysis and Applications*, 34(3):1301–1340, 2013.

[4] D. Gross and V. Nesme. Note on sampling without replacing from a finite collection of matrices. *arXiv preprint arXiv:1001.2738*, 2010.

[5] N. Halko, P.-G. Martinsson, and J. A. Tropp. Finding structure with randomness: Probabilistic algorithms for constructing approximate matrix decompositions. *SIAM review*, 53(2):217–288, 2011.

[6] J. A. Tropp. Improved analysis of the subsampled randomized hadamard transform. *Advances in Adaptive Data Analysis*, 3(01n02):115–126, 2011.

[7] J. A Tropp. User-friendly tail bounds for sums of random matrices. *Foundations of computational mathematics*, 12(4):389–434, 2012.

[8] J. A. Tropp et al. An introduction to matrix concentration inequalities. *Foundations and Trends® in Machine Learning*, 8(1-2):1–230, 2015.

[9] D. P. Woodruff et al. Sketching as a tool for numerical linear algebra. *Foundations and Trends® in Theoretical Computer Science*, 10(1–2):1–157, 2014.
